# Supplementary material for: A Deep Reinforcement Learning Chatbot (Short Version)
Source: arXiv:1801.06700 source file (2018-01-20)
Supplement: Supplementary file 1 [file appendix.tex]

\section*{Appendices}
\section{Q-learning with the Abstract Discourse Markov Decision Process}
In this appendix we describe in detail the \emph{Abstract Discourse Markov Decision Process}.

One way to quantify the differences between the supervised learning and policy gradient approaches is through the \textit{bias-variance trade-off}.
At one end of the spectrum, the \emph{Supervised AMT} policy has low variance, because it was trained with hundreds of thousands of human annotations at the level of each model response.
However, for the same reason, \emph{Supervised AMT} incurs a substantial bias, because the human annotations do not reflect the real user satisfaction for an entire conversation.
At the other end of the spectrum, \emph{Off-policy REINFORCE} suffers from high variance, because it was trained with only a few thousand dialogues and corresponding user scores.
To make matters worse, the user scores are affected by many external factors (e.g.\@ user profile, user expectations and so on) and occur at the granularity of an entire conversation.
Nevertheless, by training to directly optimize the objective metric we care about (i.e.\@ the user score) it incurs low bias.\footnote{Due to truncated importance weights, however, the \textit{Off-policy REINFORCE} training procedure is still biased.}
By utilizing a learned reward function, \emph{Supervised AMT Learned Reward} and \emph{Off-policy REINFORCE Learned Reward} suffer less from bias, but since the learned reward function has its own variance component, they are bound to suffer from higher variance.
In general, finding the optimal trade-off between bias and variance can be notoriously difficult.
To this end, we propose a novel method for trading off bias and variance by learning the policy from simulations in an approximate Markov decision process.

\textbf{Motivation}
A Markov decision process (MDP) is a framework for modeling sequential decision making~\citep{sutton1998reinforcement}.
In the general setting, an MDP is a model consisting of a discrete set of states $H$, a discrete set of actions $A$, a transition distribution function $P$, a reward distribution function $R$, and a discount factor $\gamma$.
As before, an agent aims to maximize its reward during each episode.
Let $t$ denote the time step of an episode with length $T$.
At time $t$, the agent is in state $h_t \in H$ and takes action $a_t \in A$.
Afterwards, the agent receives reward $r_t \sim R(h_t, a_t)$ and transitions to a new state $h_{t+1} \sim P(h_t | a_t)$.

Given an MDP model for open-domain conversations, there are dozens of algorithms we could apply for learning the agent's policy.
Unfortunately, such an MDP does not exist.
We could try to build one directly from the example conversations we have available, however this would require solving two extremely difficult problems.
First, we would need to learn the transition distribution $P$, which outputs the next user utterance in the dialogue given the dialogue history.
This problem is likely to be as difficult as our original problem of finding an appropriate response to the user!
Second, we would need to learn the reward distribution $R$ for each time step.
However, it is very difficult to learn to predict the user score for an entire dialogue.
Given the data we have available, estimating the reward for a single turn is bound to be even more difficult.
Instead, we propose to learn a simplified model which can serve as a substitute for the true MDP by leveraging recorded dialogues.

\begin{figure}[ht]
  \centering
  \includegraphics[scale=0.175]{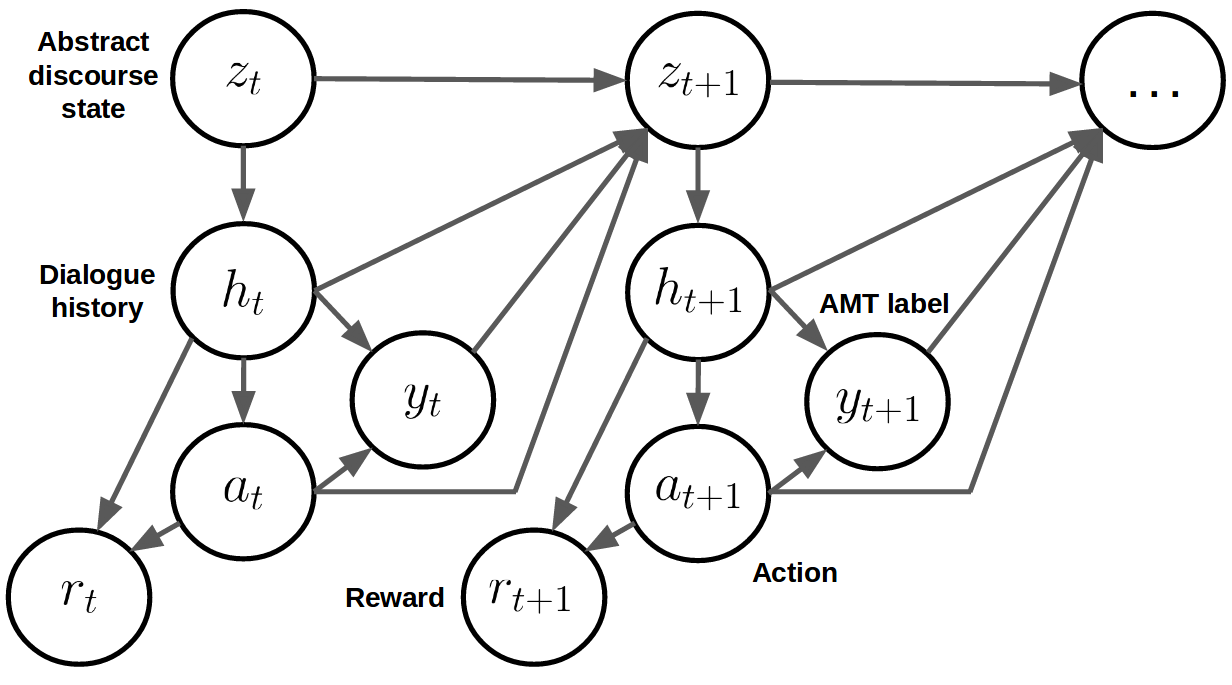}
  \caption{Probabilistic directed graphical model for the \emph{Abstract Discourse Markov Decision Process}. For each time step $t$, $z_t$ is a discrete random variable which represents the abstract state of the dialogue, $h_t$ represents the dialogue history, $a_t$ represents the action taken by the system (i.e.\@ the selected response), $y_t$ represents the sampled AMT label and $r_t$ represents the sampled reward.}
  \label{fig:approximate_mdp}
\end{figure}

\textbf{The Abstract Discourse Markov Decision Process}
The model we propose to learn is called the \emph{Abstract Discourse MDP}.
As illustrated in Figure \ref{fig:approximate_mdp}, the model follows a hierarchical structure for each time step.
At time $t$, the agent is in state $z_t \in Z$, a discrete random variable representing the \textit{abstract discourse state}.
The set $Z$ is the Cartesian product of three discrete sets:
\begin{align}
Z = Z_\text{Dialogue act} \times Z_\text{User sentiment} \times Z_\text{Generic user utterance},
\end{align}
where $Z_\text{Dialogue act}$, $Z_\text{User sentiment}$ and $Z_\text{Generic user utterance}$ are discrete sets.
The set $Z_\text{Dialogue act} = \{\text{Accept}, \text{Reject}, \text{Request}, \text{Politics}, \text{Generic Question}, \text{Personal Question}, \text{Statement}, \text{Greeting}, \text{Goodbye}, \text{Other}\}$ consists of $10$ dialogue acts, which represent the high-level intention of the user's utterance \citep{stolcke2000dialogue}.
The set $Z_\text{User sentiment} = \{\text{Negative}, \text{Neutral}, \text{Positive}\}$ consists of sentiments types.
The set $Z_\text{Generic user utterance} = \{\text{True}, \text{False}\}$ represent a binary variable, which is \textit{true} when the user utterance is generic (i.e.\@ when the user utterance only contains stop-words).
We build three deterministic classifiers, which map any dialogue history to the corresponding classes in $Z_\text{Dialogue act}$, $Z_\text{User sentiment}$ and $Z_\text{Generic user utterance}$.
We denote this mapping $f_{h \to z}$.
Although we only consider dialogue acts, sentiment and generic utterances, it is trivial to expand the \textit{abstract discourse state} with other types of discrete or real-valued variables.
%, such that $f_{h \to z}(h_t) = z_t$ where the dialogue history $h_t$ has 

Given $z_t$, the \emph{Abstract Discourse MDP} samples a dialogue history $h_t$ from a finite set of dialogue histories $H$.
In particular, $h_t$ is sampled at uniformly random from the set of dialogue histories where the last utterance is mapped to $z_t$:
\begin{align}
h_t \sim \text{Uniform}(\{h \ | \ h \in H \ \text{and} \ f_{h \to z}(h) = z_t \}).
\end{align}
In our case, $H$ is the set of all recorded dialogues.
This formally makes the \emph{Abstract Discourse MDP} a \textit{non-parametric} model, since sampling from the model requires access to the set of recorded dialogue histories $H$ which grows over time when the system is deployed in practice.
This is a useful property, because it makes it possible to continuously train the policy as new data becomes available.

Given $h_t$, the agent chooses an action $a_t$.
A reward $r_t$ is then sampled such that $r_t \sim R(h_t, a_t)$, where $R$ is a distribution function.
In our case, we use the probability function $P_{\theta}$ learned by \emph{Supervised AMT}, where we assign a reward of $-2.0$ for a \textit{very poor} response label, a reward of $-1.0$ for a \textit{poor} response label, a reward of $0.0$ for an \textit{acceptable} response label, a reward of $1.0$ for a \textit{good} response label and a reward of $2.0$ for an \textit{excellent} response label.
To reduce noise and improve convergence during training, we use the expected reward instead of a sample:
\begin{align}
r_t = P_{\theta}(y | h_t)^{\text{T}} [-2.0, -1.0, 0.0, 1.0, 2.0].
\end{align}

Next, a label $y_t$ is sampled according to $P_{\theta}$.
Finally, a new state $z_{t+1}$ is sampled:
\begin{align}
z_{t+1} \sim P_{\psi}(z | z_t, h_t, a_t, y_t).
\end{align}
where $P_{\psi}$ is the transition distribution with parameters $\psi$.
The transition distribution is parametrized by three two-layer MLP models, which take as input the same features as the scoring function, as well as 1) a one-hot vector representing the sampled response label, 2) a one-hot vector representing the dialogue act of the last user utterance, 3) a one-hot vector representing the sentiment of the last user utterance, 4) a binary variable indicating whether the last user utterance was generic, and 5) a binary variable indicating whether the last user utterance contained a wh-word.
The first MLP predicts the next dialogue act, the second MLP predicts the next sentiment type and the third MLP predicts whether the next user utterance is generic.
The dataset for training the MLPs consists of $499,757$ transitions, of which $70\%$ are used for training and $30\%$ for evaluation.
The MLPs are trained using SGD.
Due to the large number of examples, no regularization is used.
The combined three MLP models obtain a perplexity of $19.51$.
In comparison, a baseline model which, for every class, assigns the average class frequency as the output probability obtains a perplexity of $23.87$.
On average, this means that roughly $3-4$ possible $z_{t+1}$ states can be eliminated by conditioning on the previous variables $z_t, h_t, a_t$ and $y_t$.
In other words, the previous state $z_t$ and $h_t$, together with the agent's action $a_t$ has a significant impact on the future state $z_{t+1}$.
This means that an agent trained in the \emph{Abstract Discourse MDP} has the potential to learn to take into account future states of the dialogue when selecting its action.
This is contrast to policies learned using supervised learning, which do not take future dialogue states into account.

\textbf{Training}
Given the \emph{Abstract Discourse MDP}, we are now able to learn policies from simulations in the MPD.
%other reinforcement learning techniques.
We use \textit{Q-learning} with \textit{experience replay} to learn the policy, since it is simple and has been shown to be effective with policies parametrized by neural networks\citep{mnih2013playing,lin1993reinforcement}.
For experience replay, we use a memory buffer of size $1000$.
We use an $\epsilon$-greedy exploration scheme with $\epsilon=0.1$.
We experiment with discount factors $\gamma \in \{0.1, 0.2, 0.5\}$.
As before, the parameters are learned using SGD.

Training is carried out in two alternating phases.
We train the policy for $100$ episodes.
Then, we evaluate the policy for $100$ episodes w.r.t\@ average return.
Afterwards, we continue training the policy for another $100$ episodes.
During evaluation, each dialogue history is sampled from a separate set of dialogue histories $H_\text{Eval}$, which is disjoint from the set of dialogue histories $H_\text{Train}$ used at training time.
This ensures that the policy is not \textit{overfitting} our finite set of dialogue histories.
%set is disjoint from the training set
For each hyper-parameter combination, we train the policy between $400$ and $600$ episodes.
We select the policy which performs best w.r.t.\@ average return.
To keep notation brief, we call this policy \emph{Q-learning AMT}.

\newpage

\section{An Analysis of the Learned Model Selection Policies}

In this appendix, we carry out an analysis of the response model selection policies.

\begin{table}[t]
  \caption{Off-policy evaluation w.r.t.\@ expected (average) Alexa user score and number of time steps (excluding priority responses) on test set.} \label{tabel:offpolicy_evaluation}
  \small
  \centering 
    \begin{tabular}{lcc}
     \toprule
     \textbf{Policy} & \textbf{Alexa user score} & \textbf{Time steps} \\
    \midrule
    \emph{Supervised AMT} & $2.06$ & 8.19 \\
    \emph{Supervised AMT Learned Reward} & $0.94$ & 3.66 \\
    \emph{Off-policy REINFORCE} & $\mathbf{2.45}$ & 10.08 \\
    \emph{Off-policy REINFORCE Learned Reward} & $1.29$ & 5.02 \\
    \emph{Q-learning AMT} & $2.08$ & 8.28 \\ \bottomrule
    \end{tabular}
\end{table}

\textbf{Off-policy Evaluation}: One way to evaluate the model selection policies is to use the off-policy evaluation given by eq.\@ \eqref{eq:offpolicy_reinforce_evaluation}, which provides an estimate of the expected Alexa user score under each policy.\footnote{For the policies parametrized as action-value functions, we transform eq.\@ \eqref{eq:action_value_function} to eq.\@ \eqref{eq:stochastic_policy} by setting $f_\theta = Q_\theta$ and fitting the temperature parameter $\lambda$ on the development set.}
The same equation can be used to estimate the expected number of time steps per episode by substituting in a constant reward of $1.0$ per time step.
This evaluation excludes priority responses and is not directly comparable to the results in Table \ref{tabel:ab_testing_round_one}.

The result of expected Alexa user score and number of time steps per episode (excluding priority responses) are given in Table \ref{tabel:offpolicy_evaluation}.
Here we observe that the \emph{Off-policy REINFORCE} performs best followed by \emph{Q-learning AMT} and \emph{Supervised AMT} w.r.t.\@ expected user score.
\emph{Off-policy REINFORCE} reaches $2.45$, which is a major $17.8\%$ improvement over the second best performing model \emph{Q-learning AMT}.
However, this advantage should be taken with a grain of salt.
The off-policy evaluation in eq.\@ \eqref{eq:offpolicy_reinforce_evaluation} is a biased estimator since the importance weights have been truncated.
Moreover, \emph{Off-policy REINFORCE} has been trained specifically to improve on this biased estimator, while all other policies have been trained to improve upon other objective functions.
Similarly, in the evaluation w.r.t.\@ expected number of time steps, \emph{Off-policy REINFORCE} reaches the highest number of time steps followed by \emph{Q-learning AMT} and \emph{Supervised AMT}.
As before, we should take this result with a grain of salt, since this evaluation is also biased and does not take into account priority responses.
Further, it's not clear that increasing the number of time steps will increase user scores.
Regardless, \emph{Off-policy REINFORCE}, \emph{Q-learning AMT} and \emph{Supervised AMT} appear to be our prime candidates for further experiments.
This is the reason why we choose to evaluate the first two policies in the second A/B testing experiment

\begin{figure}[ht]
  \centering
  \includegraphics[scale=0.3]{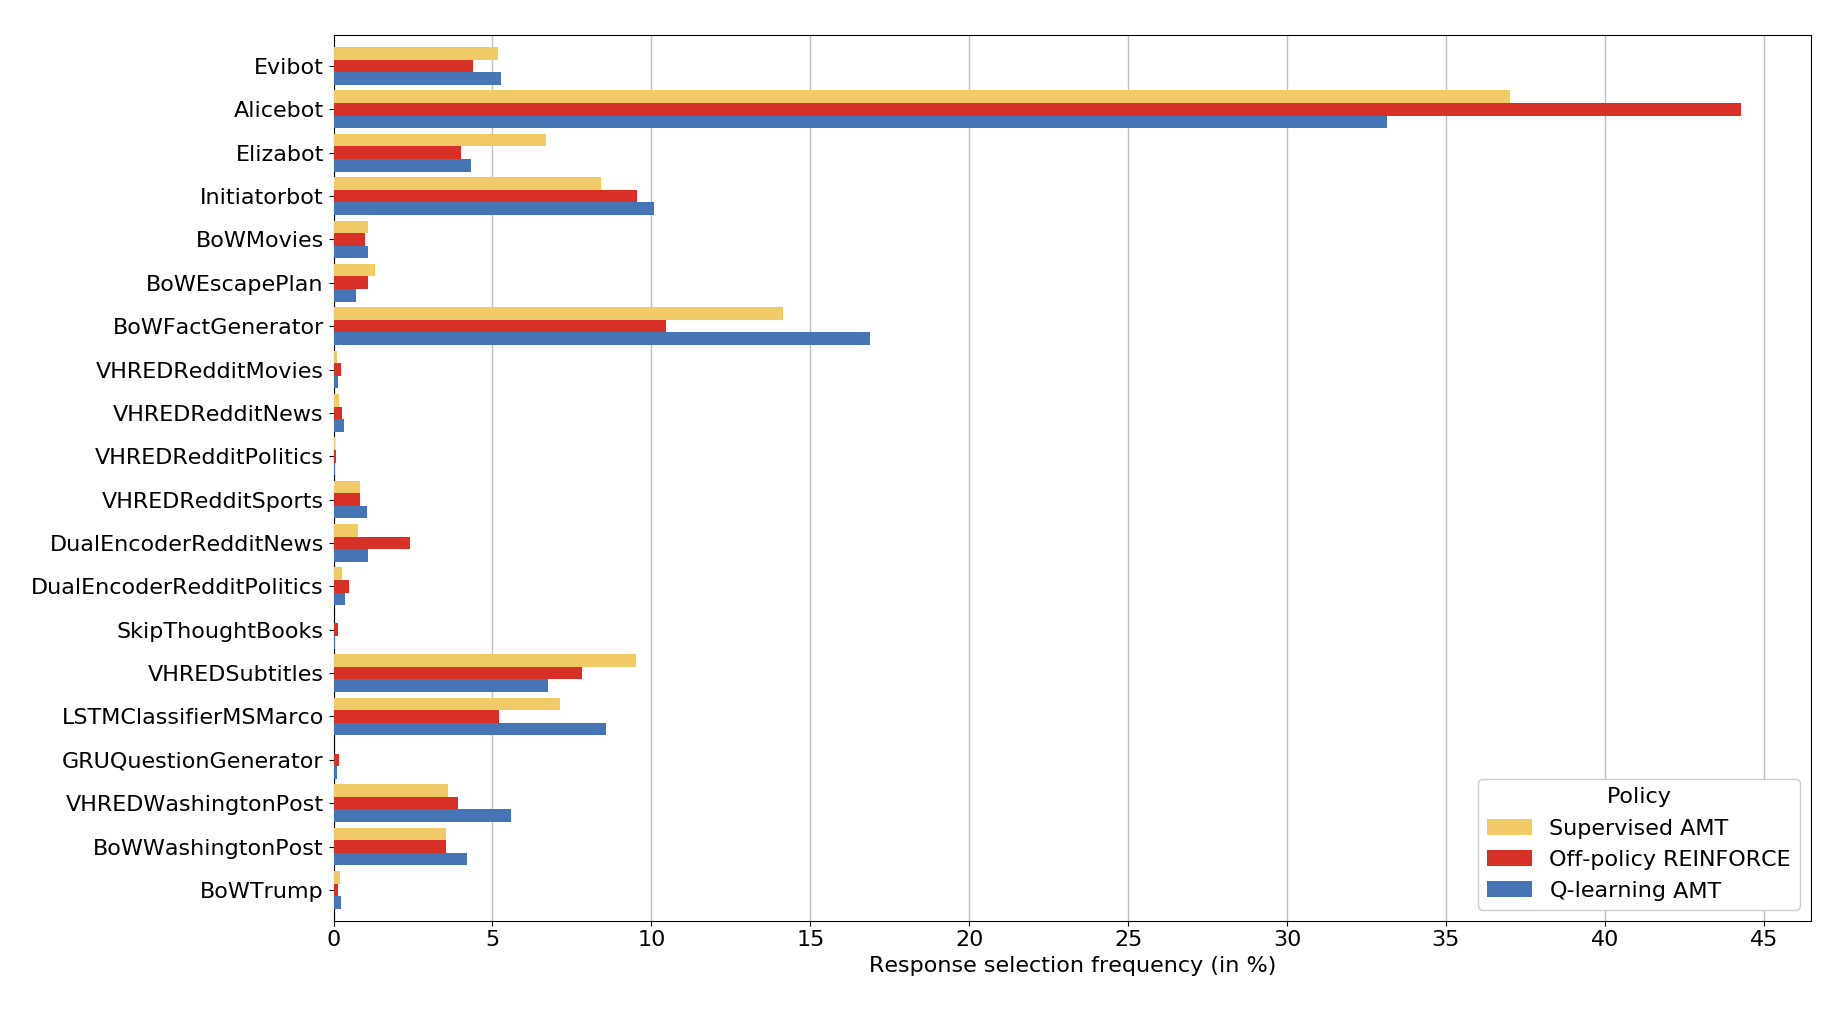}
  \caption{Response model selection probabilities across response models for \emph{Supervised AMT}, \emph{Off-policy REINFORCE} and \emph{Q-learning AMT} on the AMT label test dataset.}
  \label{fig:rl_response_model_selection_frequencies}
\end{figure}

\textbf{Response Model Selection Frequency}:
In Figure \ref{fig:rl_response_model_selection_frequencies}, we show the frequency with which \emph{Supervised AMT}, \emph{Off-policy REINFORCE} and \emph{Q-learning AMT} select different response models.
We observe that the policy learned using \emph{Off-policy REINFORCE} tends to strongly prefer \emph{Alicebot} responses over other models.
The \emph{Alicebot} responses are among the safest and most generic ones in the system, which means that \emph{Off-policy REINFORCE} has learned a highly \textit{risk averse strategy}.
On the other hand, the \emph{Q-learning AMT} policy selects \emph{Alicebot} responses substantially less often than both \emph{Off-policy REINFORCE} and \emph{Supervised AMT}.
Instead, \emph{Q-learning AMT} tends to prefer responses retrieved from Washington Post and from Google search results.
These responses are semantically richer and have the potential to engage the user more deeply in a particular topic, but they are also more risky (e.g.\@ a bad choice could derail the entire conversation.).
One possible explanation for this difference is that \emph{Q-learning AMT} was trained using simulations.
By learning online from simulations, the policy was able to explore new actions and discover new strategies lasting multiple time steps.
This would have allowed it to both experiment with more risky actions and to learn \textit{remediation} or \textit{fall-back strategies}, in cases where the risky action fails.
This might also explain its stronger preference for \emph{BoWFactGenerator}, which might serve as a fall-back strategy by outputting factual statements on the current topic.
This would have been difficult to learn for \emph{Off-policy REINFORCE}, since the sequence of actions for such strategies are sparsely observed in the data and, when they are observed, the corresponding returns (user scores) are still very noisy.

A second observation is that \emph{Q-learning AMT} has the strongest preference for \emph{Initiatorbot} among the three policies.
This could indicate that \emph{Q-learning AMT} leans towards a \textit{system-initiative strategy} (e.g.\@ a strategy where the system tries to maintain control of the conversation by asking questions, changing topics and so on).
Further analysis is needed to confirm this.

\begin{table}[t]
  \caption{Policy evaluation using the \emph{Abstract Discourse MDP} w.r.t.\@ average return, average reward per time step and average episode length on dev set ($\pm$ standard deviations). The reward function is based on \emph{Supervised AMT}.} \label{tabel:mdp_evaluation}
  \small
  \centering
    \begin{tabular}{lccc@{\hskip 0.15in}ccccc}
     \toprule
     \textbf{Policy} & \textbf{Average return} & \textbf{Average reward per time step} & \textbf{Average dialogue length} \\
    \midrule
    \emph{Random} & $-32.18 \pm 31.77$ & $-0.87 \pm 0.24$ & $34.29 \pm 33.02$ \\
    \emph{Alicebot} & $-15.56 \pm 15.61$ & $-0.37 \pm 0.16$ & $42.01 \pm 42.00$  \\
    \emph{Evibot + Alicebot} & $-11.33 \pm 12.43$ & $-0.29 \pm 0.19$ & $37.5 \pm 38.69$  \\
    \emph{Supervised AMT} & $\mathbf{-6.46 \pm 8.01}$ & $\mathbf{-0.15 \pm 0.16}$ & $\mathbf{42.84 \pm 42.92}$  \\
    \emph{Supervised AMT Learned Reward} & $-24.19 \pm 23.30$ & $-0.73 \pm 0.27$ & $31.91 \pm 30.09$ \\
    
    \emph{Off-policy REINFORCE} & $\mathbf{-7.30 \pm 8.90}$ & $\mathbf{-0.16 \pm 0.16}$ & $\mathbf{43.24 \pm 43.58}$ \\
    \parbox[c][2.65em][c]{0.225\textwidth}{\emph{Off-policy REINFORCE} \\ \protect{\hphantom{\ }} \emph{Learned Reward}} & $-10.19 \pm 11.15$ & $-0.28 \pm 0.19$ & $35.51 \pm 35.05$ \\
    \emph{Q-learning AMT} & $\mathbf{-6.54 \pm 8.02}$ & $\mathbf{-0.15 \pm 0.18}$ & $\mathbf{40.68 \pm 39.13}$ \\ \bottomrule
    \end{tabular}
\end{table}

\textbf{Abstract Discourse MDP Evaluation}: Next, we can evaluate the performance of each policy w.r.t.\@ simulations in the \emph{Abstract Discourse MDP}.
We simulate 500 episodes under each policy and evaluate it w.r.t.\@ average return, average reward per time step and dialogue length.
In addition to evaluating the five policies described earlier, we also evaluate three heuristic policies: 1) a policy selecting responses at random called \emph{Random}, 2) a policy selecting only \emph{Alicebot} responses called \emph{Alicebot},\footnote{When there are no valid \emph{Alicebot} responses, this policy selects a response at random.} and 3) a policy selecting \emph{Evibot} responses when possible and \emph{Alicebot} responses otherwise, called \emph{Evibot + Alicebot}\footnote{When there are no valid \emph{Evibot} or \emph{Alicebot} responses, this policy selects a response at random.}.
Evaluating these models will serve to validate the approximate MDP.

The results are given in Table \ref{tabel:mdp_evaluation}.
We observe that \emph{Supervised AMT} performs best w.r.t.\@ average return and average reward per time step.
However, this comes as no surprise since the reward function in the MDP is defined as \emph{Supervised AMT}.
By construction, \emph{Supervised AMT} is the policy which achieves the highest reward per time step.
On par with \emph{Supervised AMT} is \emph{Q-learning AMT}, which achieved the same $-0.15$ average reward per time step.
Next in line comes \emph{Off-policy REINFORCE}, which achieved an average reward per time step of $-0.16$.
However, \emph{Off-policy REINFORCE} also achieved the highest average dialogue length of $43.24$.
In the lower end of the spectrum comes, as expected, the \emph{Random} policy performing worst w.r.t.\@ all metrics.
In comparison, both \emph{Alicebot} and \emph{Evibot + Alicebot} perform better w.r.t.\@ all metrics, with \emph{Evibot + Alicebot} achieving the best average return and average reward per time step out of the three heuristic policies.
This validates the utility of the \emph{Abstract Discourse MDP} as an environment for training and evaluating policies.
Overall, \emph{Off-policy REINFORCE}, \emph{Q-learning AMT} and \emph{Supervised AMT} still appear to be the best performing models.

\begin{figure}[ht]
  \centering
  \includegraphics[scale=0.375]{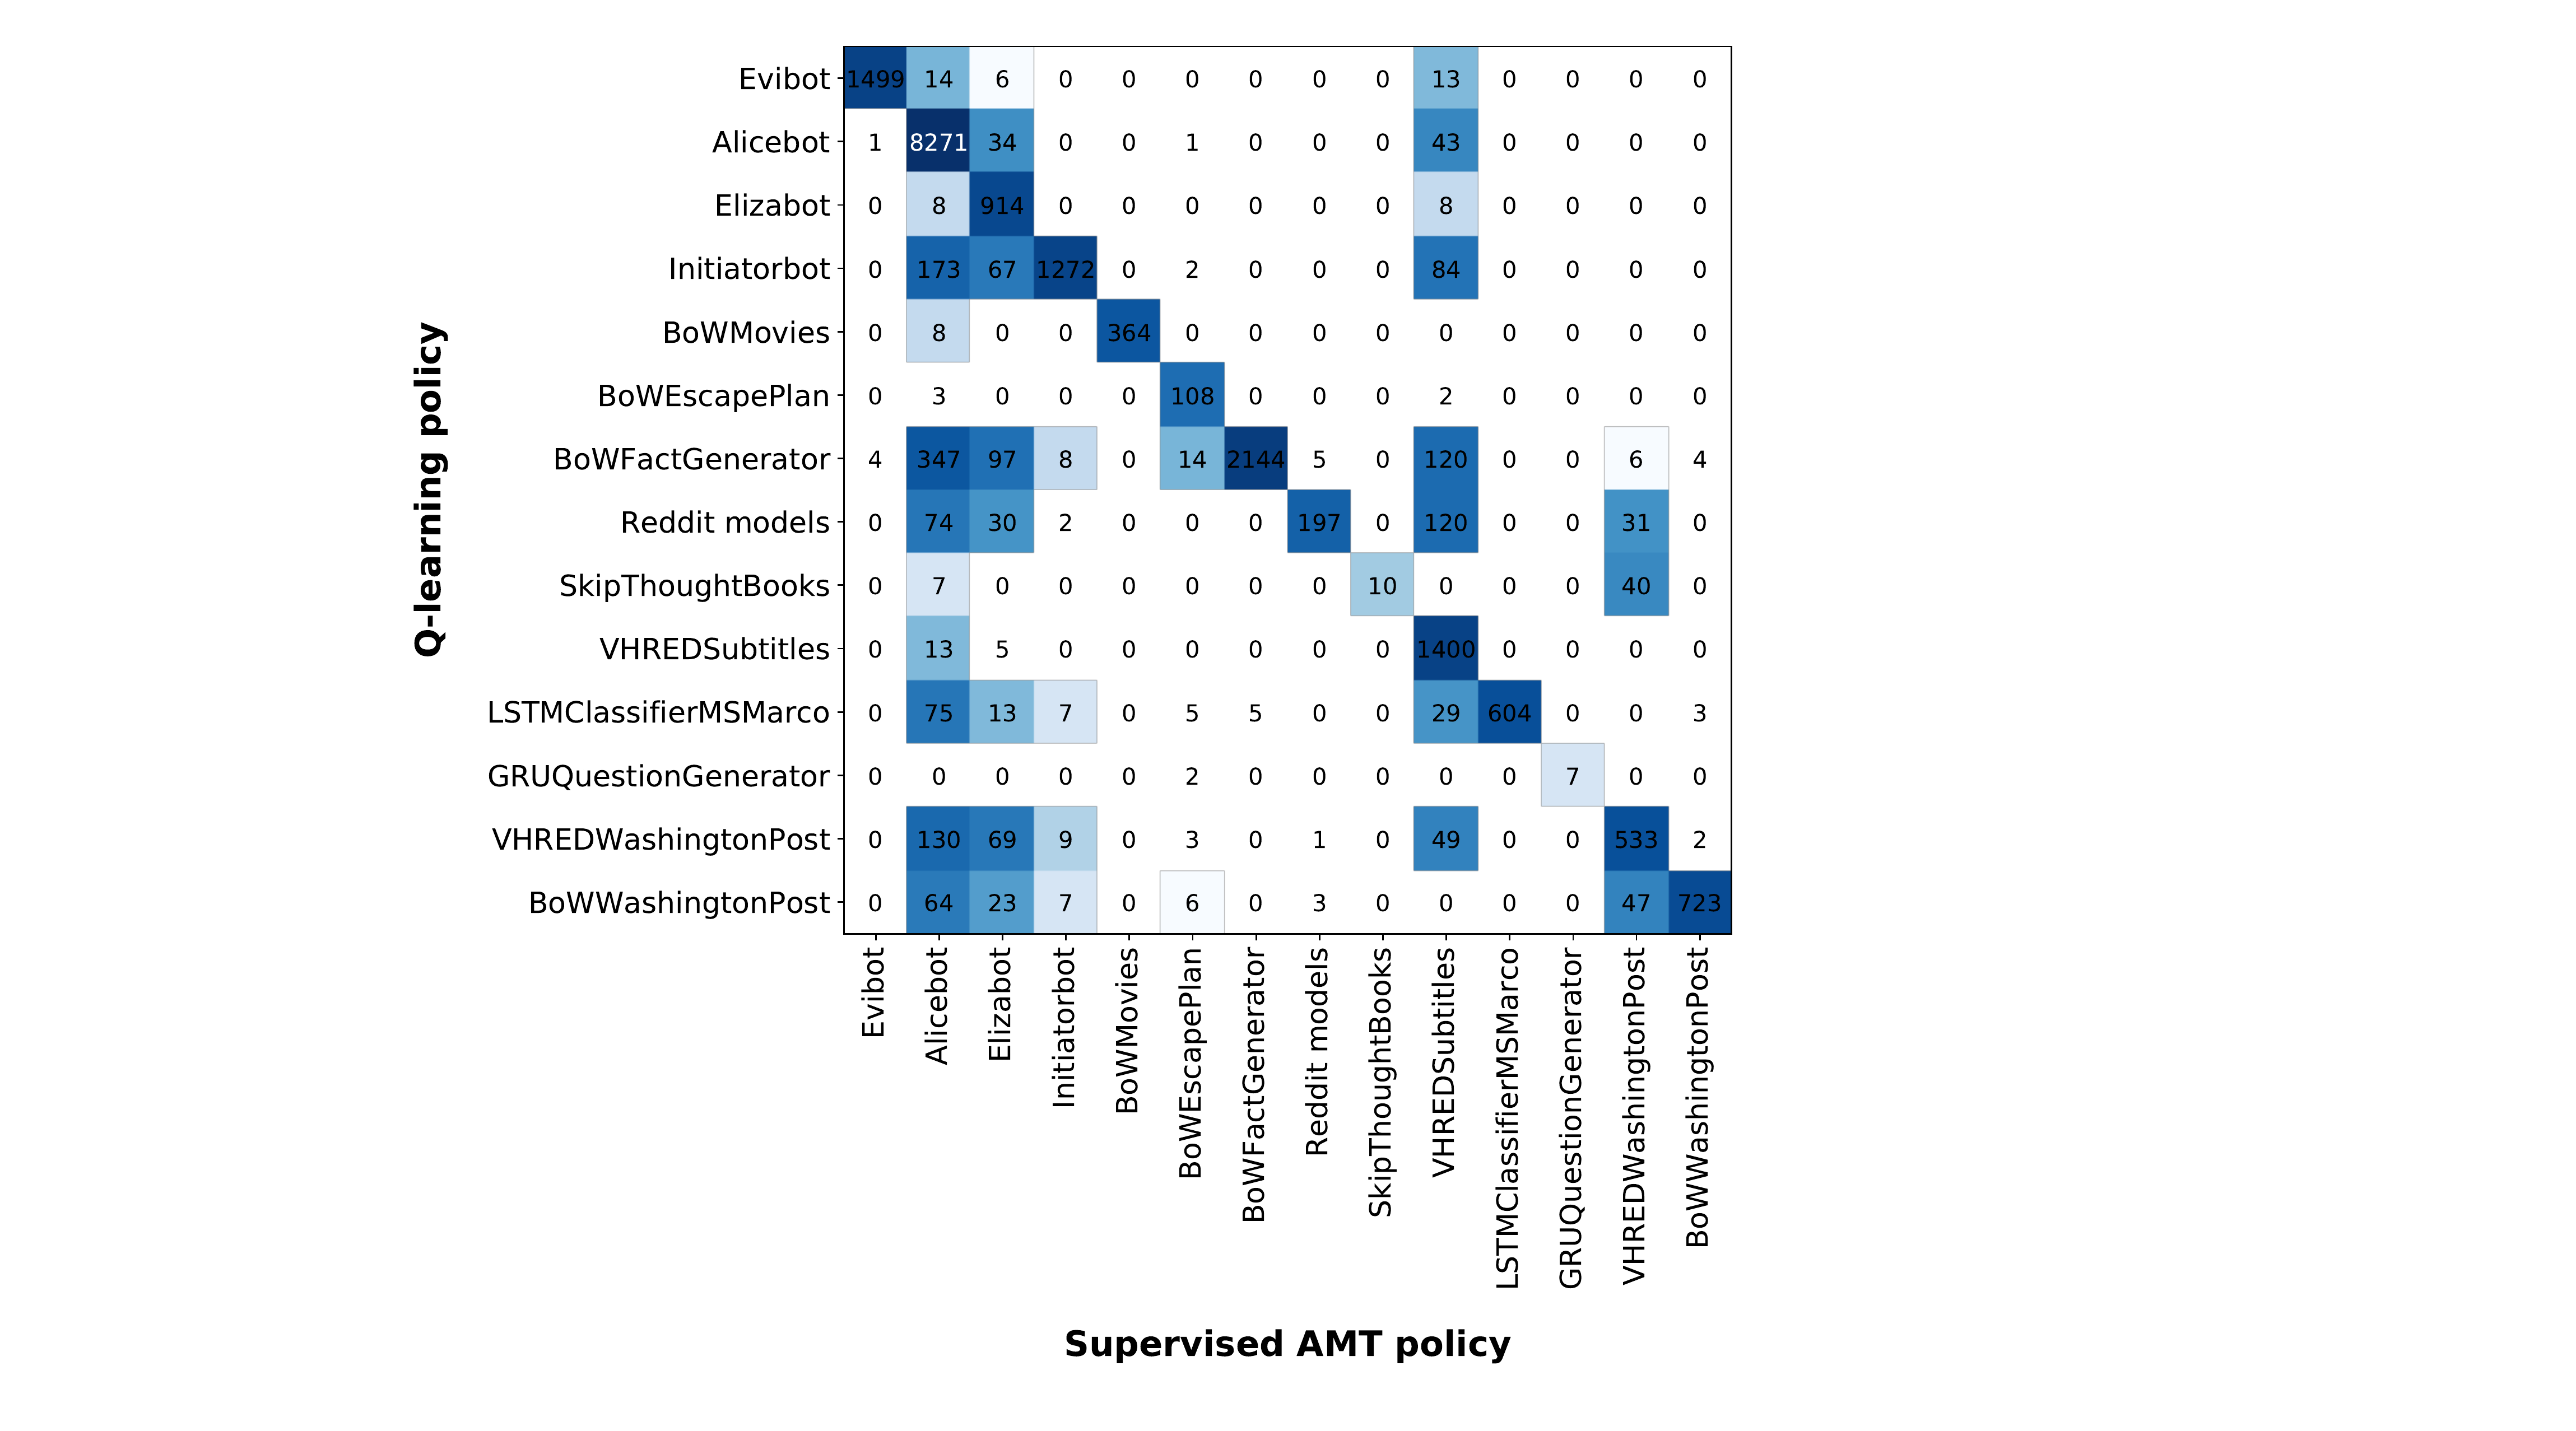}
  \caption{Contingency table comparing selected response models between \emph{Supervised AMT} and \emph{Q-learning AMT}. The cells in the matrix show the number of times the \emph{Supervised AMT} policy selected the row response model and the \emph{Q-learning AMT} policy selected the column response model. The cell frequencies were computed by simulating 500 episodes under the \emph{Q-learning AMT} policy in the \emph{Abstract Discourse MDP}. Note that all models retrieving responses from Reddit have been agglomerated into the class \emph{Reddit models}.}
  \label{fig:rl_response_model_selection_frequencies_q_learning_supervised_policy}
\end{figure}

\newpage

Finally, we compare \emph{Q-learning AMT} with \emph{Supervised AMT} one-on-one w.r.t.\@ the action taken in states from episodes simulated in the \emph{Abstract Discourse MDP}.
As shown in Figure \ref{fig:rl_response_model_selection_frequencies_q_learning_supervised_policy},
the two policies diverge w.r.t.\@ several response models.
Where \emph{Supervised AMT} would have selected generic \emph{Alicebot} and \emph{Elizabot} responses, \emph{Q-learning AMT} often selects \emph{BoWFactGenerator}, \emph{Initiatorbot} and \emph{VHREDWashingtonPost} responses.
For example, there were 347 instances where \emph{Supervised AMT} selected \emph{Alicebot} but where \emph{Q-learning AMT} selected \emph{BoWFactGenerator}.
Similarly, where \emph{Supervised AMT} would have preferred generic \emph{VHREDSubtitle} responses, \emph{Q-learning AMT} often selects responses from \emph{BoWFactGenerator}, \emph{InitiatorBot} and \emph{VHREDRedditSports}.
This supports our previous analysis showing that \emph{Q-learning AMT} has learned a more risky policy, which involves response models with semantically richer content.
